# Supplementary material for: Hybrid Spin and Anomalous Spin-Momentum Locking in Surface Elastic Waves
Source: arXiv:2308.01953 source file (2023-08-03)
Supplement: Supplementary file 1 [file Supp.pdf]

# SUPPLEMENTARY MATERIALS

# Hybrid Spin and Anomalous Spin-Momentum Locking in Surface Elastic Waves

Chenwen Yang#,[1] Danmei Zhang#,[1] Jinfeng Zhao#,[2] Wenting Gao,[1] Weitao Yuan,[3] Yang Long,[1] Yongdong Pan,[2] Hong Chen,[1] Franco Nori,[4,5,6] Konstantin Y. Bliokh,[4,7,8,*] Zheng Zhong,[2,†] and Jie Ren[1,‡]

[1]*Center for Phononics and Thermal Energy Science, China-EU Joint Lab on Nanophononics, Shanghai Key Laboratory of Special Artificial Microstructure Materials and Technology, School of Physics Science and Engineering, Tongji University, Shanghai 200092, China*

[2]*School of Aerospace Engineering and Applied Mechanics, Tongji University, Shanghai 200092, China*

[3]*School of Mechanics and Aerospace Engineering, Southwest Jiaotong University, Chengdu, Sichuan 610031, China*

[4]*Theoretical Quantum Physics Laboratory, Cluster for Pioneering Research, RIKEN, Wako-shi, Saitama 351-0198, Japan*

[5]*Center for Quantum Computing, RIKEN, Wako-shi, Saitama 351-0198, Japan*

[6]*Physics Department, University of Michigan, Ann Arbor, MI 48109-1040, USA*

[7]*Centre of Excellence ENSEMBLE3 Sp. z o.o., 01-919 Warsaw, Poland*

[8]*Donostia International Physics Center (DIPC), Donostia-San Sebastián 20018, Spain*

## 1. Transverse spin of surface electromagnetic, acoustic, and elastic waves

We consider surface waves $x$-propagating along the $z = 0$ interface between two media, as shown in Fig. 1 in the main text. First, a surface TM electromagnetic wave at an interface between the vacuum and a metal (with permittivity $\varepsilon < -1$) is known as surface plasmon-polariton [1]. Considering the vacuum ($z > 0$) part, its complex electric field has the form

$$\mathbf{E} \propto \begin{pmatrix} -i\kappa/k_x \\ 0 \\ 1 \end{pmatrix} \exp(ik_x x - \kappa z)\,, \tag{1}$$

where $k_x$ is the propagation wavenumber and $\kappa$ is the spatial decay factor. The $y$-component of the spin of this field, shown in Fig. 1(b), is [2]:

$$S \propto \mathrm{Im}(E_z^* E_x) \propto -\frac{\kappa}{k_x} \exp(-2\kappa z)\,, \tag{2}$$

* Email: kostiantyn.bliokh@riken.jp
† Email: zhongk@tongji.edu.cn
‡ Email: Xonics@tongji.edu.cn
# These authors contributed equally to this work

where we omit the subscript "$y$" for the sake of brevity.

Second, acoustic analogues of surface plasmon-polaritons can appear at an interface between air and a negative-density ($\rho < 0$) metamaterial [3, 4]. Considering the air ($z > 0$) part of such wave, its complex velocity field can be written as

$$\mathbf{v} \propto \begin{pmatrix} 1 \\ 0 \\ i\kappa/k_x \end{pmatrix} \exp(ik_x x - \kappa z)\,, \tag{3}$$

and the transverse spin density, shown in Fig. 1(c), becomes [5, 6]:

$$S \propto \mathrm{Im}(v_z^* v_x) \propto -\frac{\kappa}{k_x} \exp(-2\kappa z)\,. \tag{4}$$

Third, we consider a surface elastic (Rayleigh) wave at the surface of an isotropic solid ($z > 0$). In contrast to the purely transverse surface electromagnetic wave ($\nabla \cdot \mathbf{E} = 0$) and purely longitudinal acoustic wave ($\nabla \times \mathbf{v} = 0$), the Rayleigh wave is a *hybrid* mode including both transverse and longitudinal contributions to the displacement wavefield: $\mathbf{u} = \mathbf{u}_l + \mathbf{u}_t$ , where $\nabla \times \mathbf{u}_l = 0$ and $\nabla \cdot \mathbf{u}_t = 0$. The longitudinal and transverse parts of the complex displacement field of the Rayleigh wave can be written as [7]:

$$\mathbf{u}_l = A \begin{pmatrix} 1 \\ 0 \\ i\kappa_l/k_x \end{pmatrix} \exp(ik_x x - \kappa_l z)\,, \quad \mathbf{u}_t = B \begin{pmatrix} -i\kappa_t/k_x \\ 0 \\ 1 \end{pmatrix} \exp(ik_x x - \kappa_t z)\,. \tag{5}$$

Here the longitudinal and transverse contributions have different decay rates $\kappa_l = \sqrt{k_x^2 - k_l^2}$ and $\kappa_t = \sqrt{k_x^2 - k_t^2}$, with $k_l = \omega\sqrt{\rho/(\lambda+\mu)}$ and $k_t = \omega\sqrt{\rho/\mu}$ being the wave numbers of the longitudinal (compression) and transverse (shear) elastic bulk modes, where $\omega$ is the wave frequency, $\rho$ is the mass density of the medium, and $\lambda$ and $\mu$ are the Lamé parameters of the medium. According to the boundary conditions, the normal stress component on the surface must vanish, which yields

$$B = -i\frac{2\kappa_l k_x}{\kappa_t^2 + k_x^2} A. \tag{6}$$

The propagation constant $k_x$ of the Rayleigh wave satisfies the equation [7]

$$\frac{k_t^6}{k_x^6} - 8\frac{k_t^4}{k_x^4} + 8\frac{k_t^2}{k_x^2}\left(3 - 2\frac{k_l^2}{k_t^2}\right) - 16\left(1 - \frac{k_l^2}{k_t^2}\right) = 0. \tag{7}$$

Substituting Eqs. (5) and (6) into Eqs. (1) and (2) of the main text, the transverse spin density in the Rayleigh wave can be written as a sum of four contributions, $S = S_{ll} + S_{tt} + S_{lt} + S_{tl}$:

$$S_{ll} \propto \mathrm{Im}(u_{l\,z}^* u_{l\,x}) = -|A|^2 \frac{\kappa_l}{k_x} e^{-2\kappa_l z}, \quad S_{tt} \propto \mathrm{Im}(u_{t\,z}^* u_{t\,x}) = -|B|^2 \frac{\kappa_t}{k_x} e^{-2\kappa_t z}, \tag{8}$$

$$S_{lt} \propto \mathrm{Im}(u_{l\,z}^* u_{t\,x}) = \mathrm{Im}(AB^*)\,\frac{\kappa_t \kappa_l}{k_x^2}\, e^{-(\kappa_t+\kappa_l)z}, \quad S_{tl} \propto \mathrm{Im}(u_{t\,z}^* u_{l\,x}) = \mathrm{Im}(AB^*)\, e^{-(\kappa_t+\kappa_l)z}. \tag{9}$$

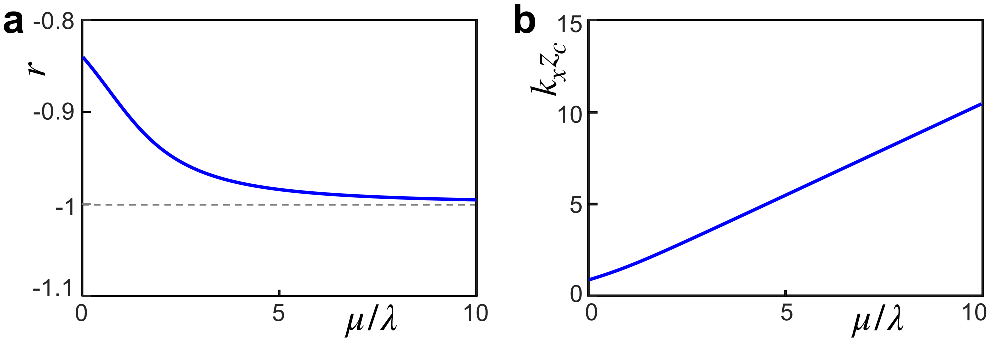


**Supplementary Figure 1.** **(a)** The ratio $r$ of the 'pure' and 'hybrid' contributions to the Rayleigh-wave spin at the surface ($z = 0$), Eq. (10), versus the ratio of the Lamé parameters, $\mu/\lambda$. **(b)** The critical depth $z_c$, Eq. (11), where the Rayleigh-wave spin vanishes and changes its sign, versus $\mu/\lambda$. Note that $\mu/\lambda \simeq 0.46$ for the aluminium used in our experiments ($\lambda = 5.5 \times 10^{10}$, $\mu = 2.5 \times 10^{10}$).

From Eq. (6) one can see that the 'hybrid' contributions (9) have opposite signs as compared to the 'pure' contribution (8). Moreover, since $\kappa_t < \kappa_l$, the hybrid contributions decay with $z$ faster than the pure transverse one. The normalized spin contributions are obtained via division of the expressions (8) and (9) by $|\mathbf{u}|^2/2$.

At the surface $z = 0$, the ratio of the pure and hybrid contributions to the Rayleigh-wave spin is:

$$r \equiv \frac{S_{ll} + S_{tt}}{S_{lt} + S_{tl}} = -\frac{(|A|^2\kappa_l + |B|^2\kappa_t)k_x}{\mathrm{Im}(AB^*)\,(k_x^2 + \kappa_l\kappa_t)}. \tag{10}$$

This ratio depends only on the ratio of the Lamé parameters, $\mu/\lambda$, as shown in Fig. S1(a). Since $|r| < 1$, the hybrid contributions dominate at the surface and determine the anomalous sign of the transverse spin there, see Figs. 1(d) and 2 in the main text. However, with $z$ growing, the pure contributions (mostly the transverse one) start to prevail, so that the total spin vanishes and flips its sign at a certain $z = z_c$. By solving the equation $S_{ll} + S_{tt} + S_{lt} + S_{tl} = 0$ with respect to $z$ and neglecting negative solutions we find

$$z_c = \frac{1}{\kappa_l - \kappa_t} \ln\left(\frac{k_x^2 + \kappa_t^2}{2\kappa_l\kappa_t}\right). \tag{11}$$

The dimensionless quantity $k_x z_c$ depends only on the ratio $\mu/\lambda$, as shown in Fig. S1(b).

## 2. Extraction of the longitudinal and transverse contributions to the Rayleigh-wave field from experimental measurements

Importantly, only the total displacement field $\mathbf{u}$ and the corresponding total spin $S$ are directly measurable quantities, while the transverse/longitudinal/hybrid contributions there are theoretical concepts. Nonetheless, one can retrieve these contributions from the experimental measurements of the total Rayleigh-wave field and its *gradients* at a given point. Using $\mathbf{u} = \mathbf{u}_l + \mathbf{u}_t$ and Eqs. (5),

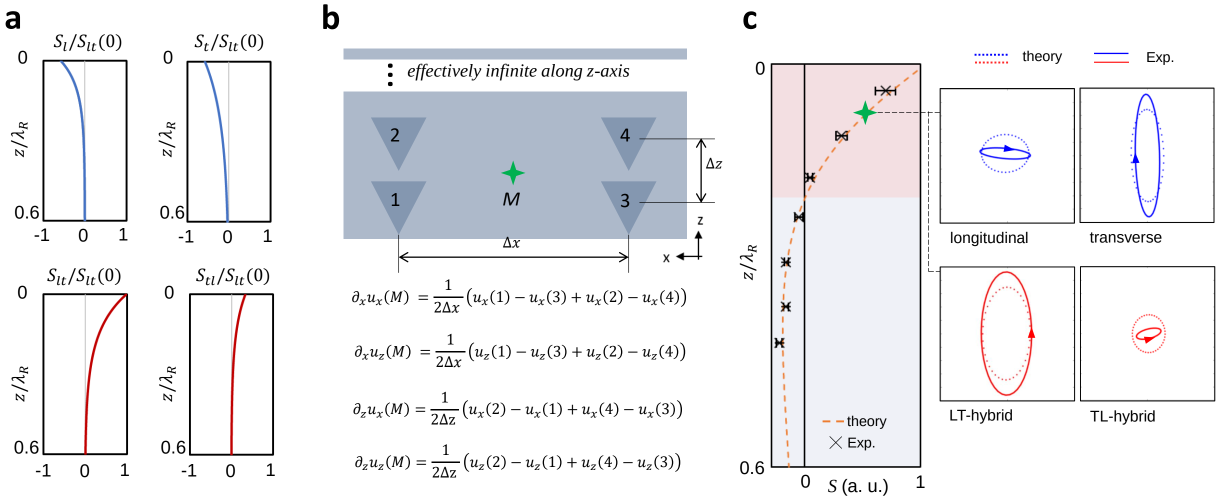


**Supplementary Figure 2.** **(a)** Different spin contributions in the Rayleigh wave. Spin reversal along the z-axis due to the faster decay of the summation of the hybrid contributions compared to the summation of pure ones. **(b)** Reconstruction of the longitudinal ($\mathbf{u}_l$) and transverse ($\mathbf{u}_t$) contributions to the Rayleigh-wave field $\mathbf{u}$, as well as of the mixed fields $\mathbf{u}_{lt}$ and $\mathbf{u}_{tl}$, from the finite-difference measurements of the total field gradients in the vicinity of a chosen point $M$ (see explanations in the text). **(c)** Here we give $S$ on the left panel as a supplement to the results of $s$ in the main text. The position of point $M$ is marked as a green cross star. The right panel contains the experimentally retrieved and theoretically calculated elliptical polarizations.

we express the transverse and longitudinal field components as

$$u_{lx} = \frac{1}{1-\kappa_l/\kappa_t}\left(\frac{\partial_x u_x}{ik} + \frac{\partial_z u_x}{\kappa_t}\right), \quad u_{tx} = \frac{1}{1-\kappa_t/\kappa_l}\left(\frac{\partial_x u_x}{ik} + \frac{\partial_z u_x}{\kappa_l}\right),$$
$$u_{lz} = -\frac{\partial_z u_z + iku_{tx}}{\kappa_l}, \qquad u_{tz} = \frac{\partial_x u_z + \kappa_l u_{lx}}{ik}. \tag{12}$$

To measure the $(x, z)$ gradients of the total displacement field $\mathbf{u}$ in a point $M$, we arranged four triangular pillars around this point, as shown in Fig. S2(b). Measuring the total field at the four pillars, we calculate the field gradients in the finite-difference approximation, Fig. S2(b). Substituting these results into Eqs. (12), we calculate the components of the longitudinal and transverse fields $\mathbf{u}_l$ and $\mathbf{u}_t$, as well as the 'mixed' fields $\mathbf{u}_{lt} = (u_{l\,z}, u_{t\,x})$ and $\mathbf{u}_{tl} = (u_{t\,z}, u_{l\,x})$ corresponding to the hybrid contributions to the Rayleigh-wave spin, see Fig. 2(a) in the main text. The comparison of the experimentally retrieved and theoretically calculated elliptical polarizations of the fields $\mathbf{u}_l$, $\mathbf{u}_t$, $\mathbf{u}_{lt}$, and $\mathbf{u}_{tl}$ is shown in Fig. S2(c). In the experiment, the position of the point M is $z = 5.5$ mm, $\Delta z = 5$ mm, and $\Delta x = 20$ mm, the frequency of the Rayleigh wave is 35 kHz. Taking into account the approximate character of this approach and the non-ideal character of the measured wavefield, the agreement is quite good.

This four-point experiment aims to retrieve the transverse and longitudinal displacement vectors from the experimental data, which can then be compared with the theoretical calculations. This is important for understanding different contributions to the spin angular momentum. In this

manner, we can not only observe the total spin of elastic waves, but also retrieve and analyse its "pure" and "hybrid" parts.

## 3. Fields and spin contributions in Lamb modes

We now consider symmetric (S) and antisymmetric (A) elastic Lamb modes in a solid plate ranging from $z = -d$ to $z = d$ and infinite along the $x$-axis. Akin to Eq. (5), the longitudinal and transverse field contributions to these modes can be written as:

$$\mathbf{u}_{Sl} = A_S \begin{pmatrix} i\cosh(\kappa_{lS} z) \\ 0 \\ \frac{\kappa_{lS}}{k_S}\sinh(\kappa_{lS} z) \end{pmatrix} e^{ik_S x}, \quad \mathbf{u}_{St} = B_S \begin{pmatrix} -\frac{\kappa_{tS}}{k_S}\cosh(\kappa_{tS} z) \\ 0 \\ i\sinh(\kappa_{tS} z) \end{pmatrix} e^{ik_S x}, \tag{13}$$

$$\mathbf{u}_{Al} = A_A \begin{pmatrix} i\sinh(\kappa_{lA} z) \\ 0 \\ \frac{\kappa_{lA}}{k_A}\cosh(\kappa_{lA} z) \end{pmatrix} e^{ik_A x}, \quad \mathbf{u}_{At} = B_A \begin{pmatrix} -\frac{\kappa_{tA}}{k_A}\sinh(\kappa_{tA} z) \\ 0 \\ i\cosh(\kappa_{tA} z) \end{pmatrix} e^{ik_A x}. \tag{14}$$

Here $k_S$ and $k_A$ are the propagation constants of the S and A modes, which can be found from the characteristic equation [8], whereas $\kappa_{lS} = \sqrt{k_S^2 - k_l^2}$, $\kappa_{tS} = \sqrt{k_S^2 - k_t^2}$, $\kappa_{lA} = \sqrt{k_A^2 - k_l^2}$, and $\kappa_{tA} = \sqrt{k_A^2 - k_t^2}$. From the boundary conditions, the amplitudes of the longitudinal and transverse fields are related as:

$$B_S = \frac{2i\kappa_{lS} k_S \sinh(\kappa_{lS} d)}{(\kappa_{tS}^2 + k_S^2)\sinh(\kappa_{tS} d)} A_S\,, \quad B_A = \frac{2i\kappa_{lA} k_A \cosh(\kappa_{lA} d)}{(\kappa_{tA}^2 + k_A^2)\cosh(\kappa_{tA} d)} A_A\,. \tag{15}$$

We consider only the lowest-order modes S0 and A0, where $k_A > k_S$ for the aluminium strip in our experiments. We also work in the frequency range below the cut-off frequency of the A1 mode. In this case $k_A > k_t > k_l$ and $k_t > k_S > k_l$, so that $\kappa_{tS}$ becomes imaginary, while $B_S/A_S$ is real. Substituting Eqs. (13) and (14) into Eqs. (1) and (2) of the main text, we obtain the four contributions to the transverse spin density in the S0 and A0 Lamb modes:

$$S_{llS} \propto |A_S|^2 \frac{\kappa_{lS}}{2k_S}\sinh(2\kappa_{lS} z), \qquad S_{ttS} \propto |B_S|^2 \frac{-i\kappa_{tS}}{2k_S}\sin(-2i\kappa_{tS} z), \tag{16}$$
$$S_{ltS} \propto -\mathrm{Re}(A_S^* B_S)\frac{-i\kappa_{lS}\kappa_{tS}}{k_S^2}\cos(-i\kappa_{tS} z)\sinh(\kappa_{lS} z), \; S_{tlS} \propto -\mathrm{Re}(A_S^* B_S)\cosh(\kappa_{lS} z)\sin(-i\kappa_{tS} z),$$

$$S_{llA} \propto |A_A|^2 \frac{\kappa_{lA}}{2k_A}\sinh(2\kappa_{lA} z), \qquad S_{ttA} \propto |B_A|^2 \frac{\kappa_{tA}}{2k_A}\sinh(2\kappa_{tA} z), \tag{17}$$
$$S_{ltA} \propto -\mathrm{Im}(A_A^* B_A)\cosh(\kappa_{tA} z)\sinh(\kappa_{lA} z), \;\; S_{tlA} \propto -\mathrm{Im}(A_A^* B_A)\frac{\kappa_{lA}\kappa_{tA}}{k_A^2}\cosh(\kappa_{lA} z)\sinh(\kappa_{tA} z).$$

One can see that, similarly to the Rayleigh-wave case, the 'pure' and 'hybrid' contributions to the spin have opposite signs. The $z$-distributions of the total spin density in the S0 and A0 Lamb modes, as well as its 'pure' and 'hybrid' parts, are shown in Figs. 3 and 4(a) in the main text. The

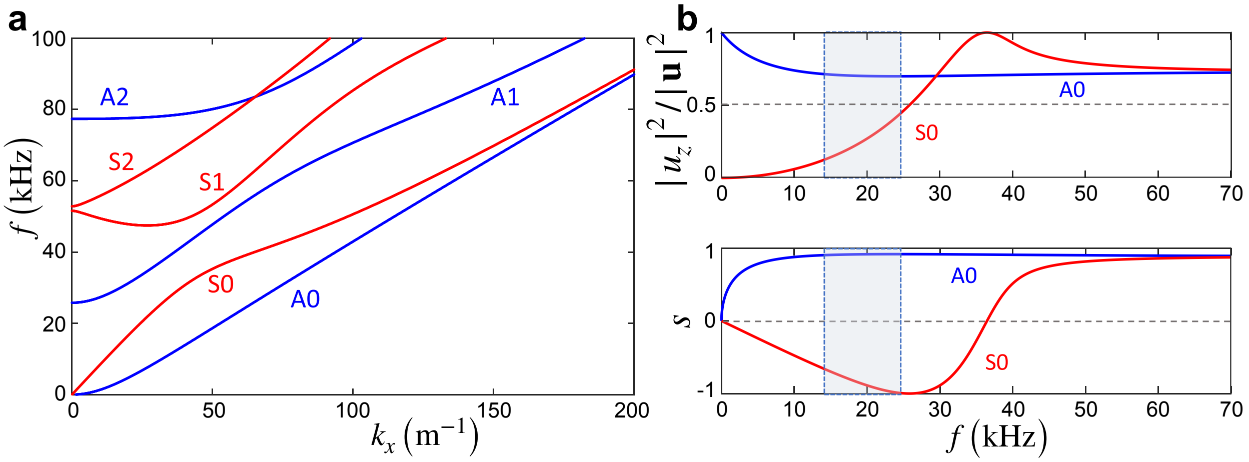


**Supplementary Figure 3.** **(a)** Dispersions of the symmetric and antisymmetric Lamb modes in an aluminium strip with $d = 3\,\mathrm{cm}$. **(b)** The frequency dependencies of the ratio of $|u_z|^2/|\mathbf{u}|^2$ and the normalized spin density $s$ at $z = -d$ in the A0 and S0 modes. The light blue area indicates the frequency range of the simulations in Fig. S4.

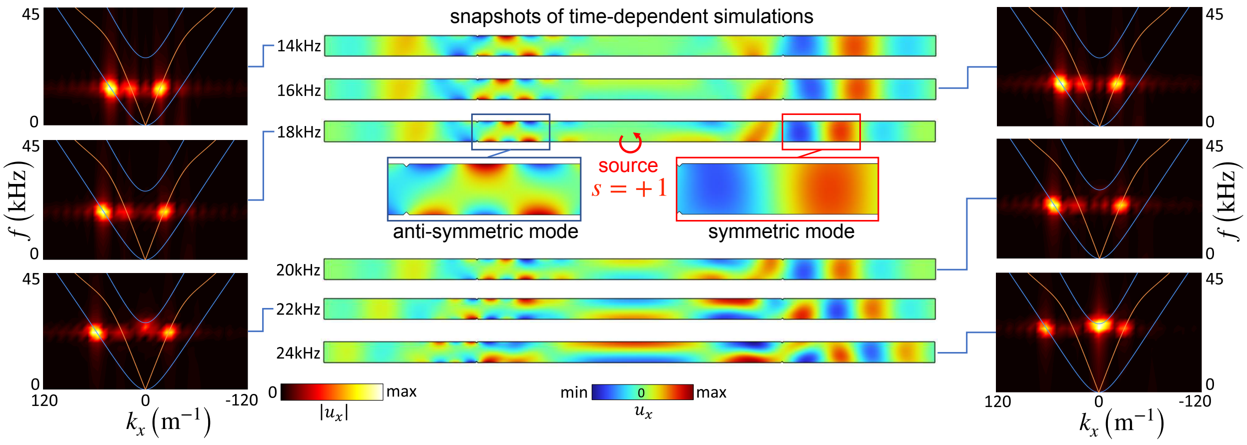


**Supplementary Figure 4.** Numerical simulations of the excitation of the Lamb waves in an aluminium strip with $d = 3\,\mathrm{cm}$ by a circularly polarized source with $s = +1$ located at $z = -d$. The results are shown for different central frequencies $f = 14\text{–}24\,\mathrm{kHz}$.

normalized spin contributions are obtained dividing the expressions (16) and (17) by $|\mathbf{u}_S|^2/2$ and $|\mathbf{u}_A|^2/2$, respectively.

## 4. Frequency-dependent polarization properties of the Lamb modes

The dispersions of the Lamb modes, calculated from the characteristic equations [8] for an aluminium strip with $d = 3\,\mathrm{cm}$, are shown in Fig. S3(a). In this work we focus on the A0/S0 modes and avoid the excitation of higher modes. Therefore, the central frequency of the pulses used in our experiments was below the cutoff frequency $f_c \simeq 25\,\mathrm{kHz}$ of the A1 mode.

The displacement field $\mathbf{u}$ of the A0/S0 mode at the edge ($z = -d$) is elliptically polarized. Im-

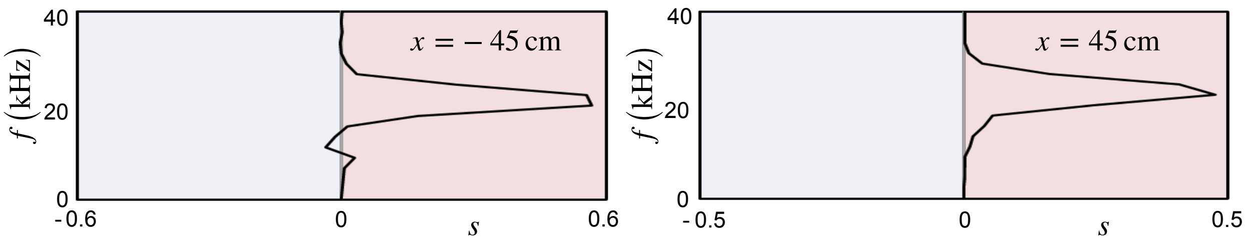


**Supplementary Figure** 5. Experimentally measured spectra of the normalized spin density $s$ (at $z = -d$) in the Lamb waves excited by a circularly-polarized source ($s = +1$) and propagating in the $+x$ and $-x$ directions.

portantly, the properties of the polarization ellipse, and hence the spin $s$ at the edge, are frequency-dependent. To characterize this dependence, in Fig. S3(b) we plot the ratio $\gamma = |u_z|^2/|\mathbf{u}|^2 \in (0, 1)$ and the normalized spin $s = 2\text{Im}(u_z^* u_x)/|\mathbf{u}|^2$ versus frequency $f = \omega/2\pi$. The value $\gamma = 0.5$ corresponds to a circular polarization (maximum normalized spin $|s| = 1$), whereas $\gamma = 0$ and $1$ correspond to linear polarizations (vanishing spin $s = 0$). In the limit of low frequencies $f \to 0$, the polarizations of the A0/S0 modes are linear and their spins vanish at the edge. As the frequency grows, the polarizations become elliptical, with opposite rotation directions, and the spins of the S0 and A0 modes at the edge, achieve almost maximum opposite values $s_A \simeq 1$ and $s_S \simeq -1$ for frequencies $f \simeq 20-25$ kHz. That is why we chose the central frequency $f = 20$ kHz in our experiments on the spin-controlled directional excitation of the Lamb modes, see Fig. 4 in the main text.

Remarkably, the edge spin of the S0 mode vanishes and changes its sign at $f \simeq 37$ kHz. For higher frequencies, the polarization-spin properties of the A0 and S0 modes coincide with each other. This is because both of these modes can be approximated by a pair of Rayleigh waves at the upper and lower edges of the strip [8]. This leads to the same dispersion relations and polarizations.

In addition to the experimental measurements shown in Fig. 4 in the main text, we performed numerical simulations of the excitation of the Lamb waves by a circularly-polarized source with $s = +1$ at the $z = -d$ edge. Results of these simulations with the parameters corresponding to the experimental one and different central frequencies $f = 14-24$ kHz are shown in Fig. S4. One can see an excellent agreement with the experimental results for $f = 20$ kHz, Fig. 4(c) in the main text. In addition, one can see that lower central frequencies cause an admixture of the S0 mode propagating in the $+x$ direction, whereas higher frequencies cause an admixture of the higher-order A1 mode.

Finally, in our experiment we checked that the positive spin $s > 0$ generated by the source is transferred by the excited Lamb modes propagating in the $+x$ and $-x$ directions. For this, we measure the frequency spectra of the spin $s$ at distances $x = 45$ cm and $x = -45$ cm from the source. Figure S5 clearly shows that both propagating Lamb waves carry positive spins $s > 0$.

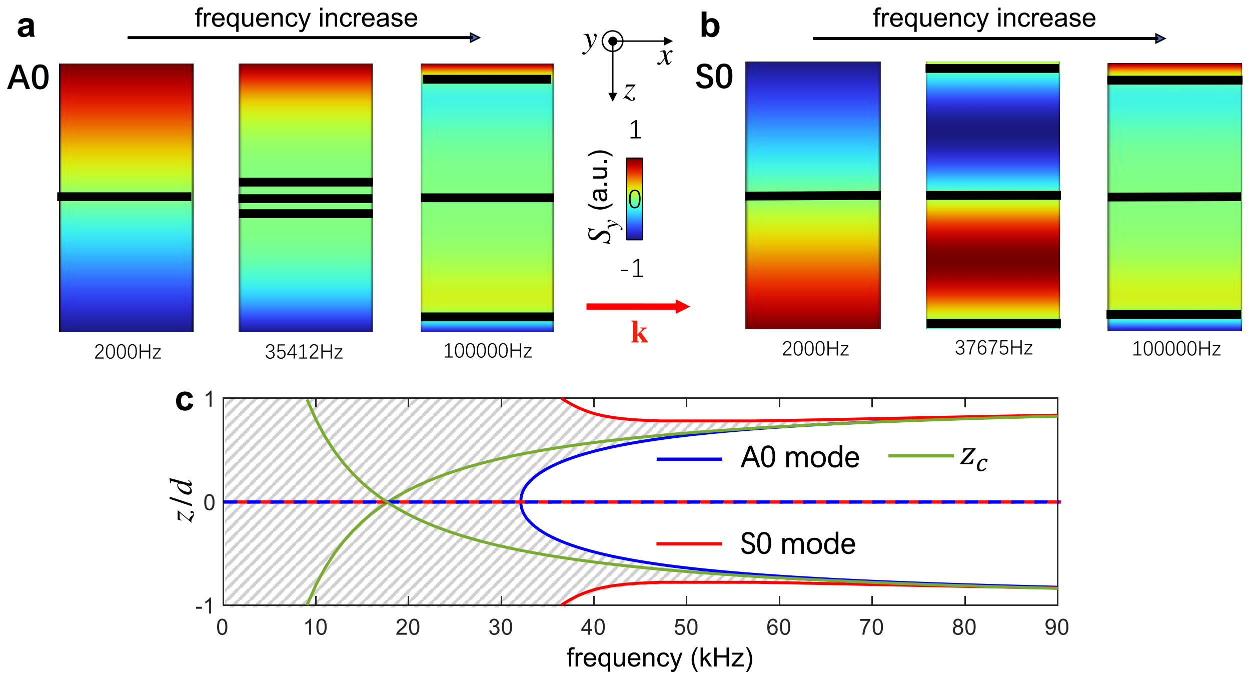


**Supplementary Figure** 6. The zero-spin ($S_y = 0$) planes in the A0 and S0 Lamb modes. These planes are shown in black in the panels **(a)** and **(b)** against the spin-density background. The central zero-spin plane is always present at $z = 0$ due to the symmetry. Two additional planes appear in the center/edges for the A0/S0 mode and move to the Rayleigh-wave position (at the distances $z_c$ from the edges) as the frequency increases. The panel **(c)** shows the frequency dependences of the spin zeros for the A0 mode, S0 mode, and the Rayleigh waves ($z_c$ distances from the edges). The shaded region corresponds to the opposite spin signs in the A0 and S0 modes.

## 5. Zero spin planes in Rayleigh-Lamb mode

As shown in Fig. 3, the spin properties of the A0 and S0 modes gradually become the same as the frequency increases. This is because at high frequencies, the skin depth of a pair of surface modes is much shorter than the width of the solid strip, causing the two surface modes to become independent of each other. Thus, both the A0 and S0 modes can be regarded as a pair of Rayleigh modes at high frequencies.

Similar to the critical depth $z_c$ in Rayleigh waves, the Lamb modes also contain planes where the elastic spin vanishes. In the main text, we show that the central $z = 0$ plane of a solid strip is such a zero-spin plane. This is determined by the symmetry of the plate, which requires that $s(z) = -s(-z)$. As the frequency increases, two additional zero-spin planes appear. These zero planes gradually approach positions at the $z_c$ distances from the plate surfaces, as shown in Fig. 6.


[1] S. A. Maier, *Plasmonics: Fundamentals and Applications* (Springer, 2007).

[2] K. Y. Bliokh, D. Smirnova, and F. Nori, Quantum spin Hall effect of light, Science **348**, 1448 (2015).

[3] M. Ambati, N. Fang, C. Sun, and X. Zhang, Surface resonant states and superlensing in acoustic meta-

materials, Phys. Rev. B **75**, 195447 (2007).

[4] C. M. Park, J. J. Park, S. H. Lee, Y. M. Seo, C. K. Kim, and S. H. Lee, Amplification of acoustic evanescent waves using metamaterial slabs, Phys. Rev. Lett. **107**, 194301 (2011).

[5] C. Shi, R. Zhao, Y. Long, S. Yang, Y. Wang, H. Chen, J. Ren, and X. Zhang, Observation of acoustic spin, Natl. Sci. Rev. **6**, 707 (2019).

[6] K. Y. Bliokh and F. Nori, Transverse spin and surface waves in acoustic metamaterials, Phys. Rev. B **99**, 020301(R) (2019).

[7] K. F. Graff, *Wave Motion in Elastic Solids* (Ohio State University Press, 1975).

[8] J. L. Rose, *Ultrasonic Guided Waves in Solid Media* (Cambridge University Press, Cambridge, 2014).
